# Supplementary material for: An Evolved Universal Transformer Memory
Source: arXiv:2410.13166 source file (2025-02-13)
Supplement: Supplementary file 1 [file appendix.tex]

\appendix
\section{Authors Contributions}
\label{sec:author_contributions}
